# Supplementary material for: Quantum size effects, multiple Dirac cones and edge states in ultrathin Bi(110) films
Source: arXiv:2106.13943 source file (2021-06-26)
Supplement: Supplementary file 1 [file Supporting_Information.pdf]

# Quantum Size Effects, Multiple Dirac Cones and Edge States in Ultrathin Bi(110) Films

Asish K. Kundu[1, *], Genda Gu[1], and Tonica Valla[1, ‡]

[1]Condensed Matter Physics and Materials Science Department, Brookhaven National Laboratory, Upton, New York 11973, USA

* akundu@bnl.gov
‡ valla@bnl.gov

## Fermi surface and constant energy contour of 3 BL Bi film:

In figure. S1, the 2D curvature plots of the FS and the constant energy contour at -50 meV for the 3 BL films are shown. The red square represents one quadrant of the SBZ. Panels (c) and (d) are the same as (a) and (b), with the 1D Fermi surfaces marked by white dashed lines. These 1D FSs are more prominent in the direction parallel with the $k_x$, suggesting that the islands have preferential growth direction along $k_x$.

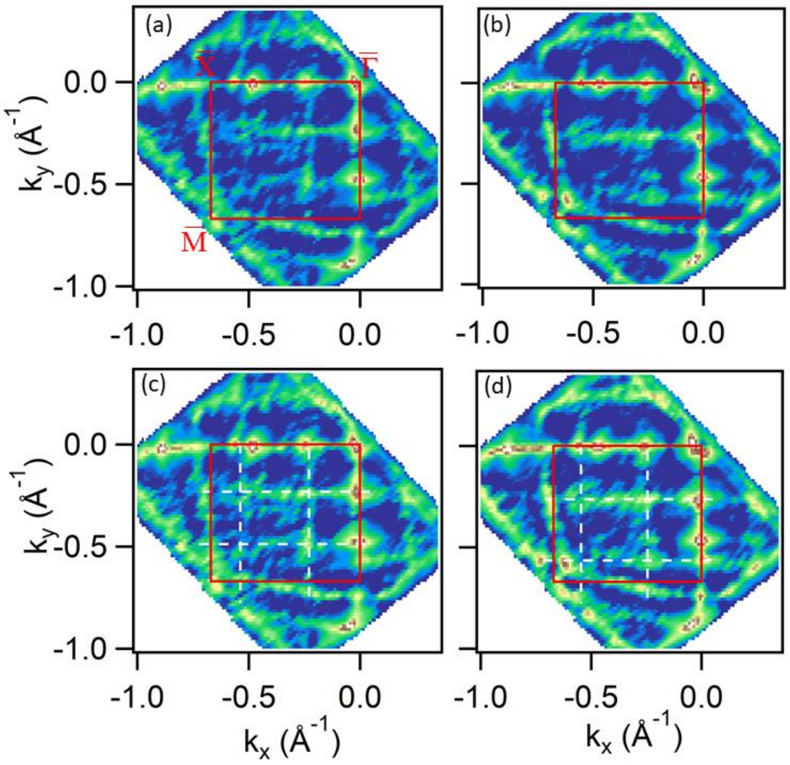


Figure S1. 2D curvature plot of FS and the constant energy contour at -50 meV for the 3 BL Bi films. (a) FS and (b) constant energy contour at -50 meV. (c), (d) the same as (a), (b), but with the 1D FSs marked by the white dashed lines.

## Comparison between experimental and theoretical dispersions accounting various structure of Bi(110) films:

In figure S2, the comparison between experimental and theoretical dispersions along $\bar{\Gamma} - \bar{M}$ symmetry directions of Bi(110) SBZ accounting bulk-like and BP-like Bi(110) films are presented. In panel (a), electronic states 2, 3 and 4, 5 originates from the 6 BL and 8 BL islands of Bi(110) films, as already discussed in the main text. Panel (c) and (d) are the theoretical dispersions for 6 BL and 8 BL Bi(110) films, respectively, accounting for both bulk [8] and BP-like [24] structure. The experimental energy separation between the states 2 and 3 is closer to the calculations with the BP-like film structure (panel (b)). The same is true for the states 4 and 5 (panel (c)). Also, the electronic states inside the red square in panel (a) can only be reproduced in 8 BL films with BP structure. Therefore, the structure of even bilayer films is likely the BP-like.

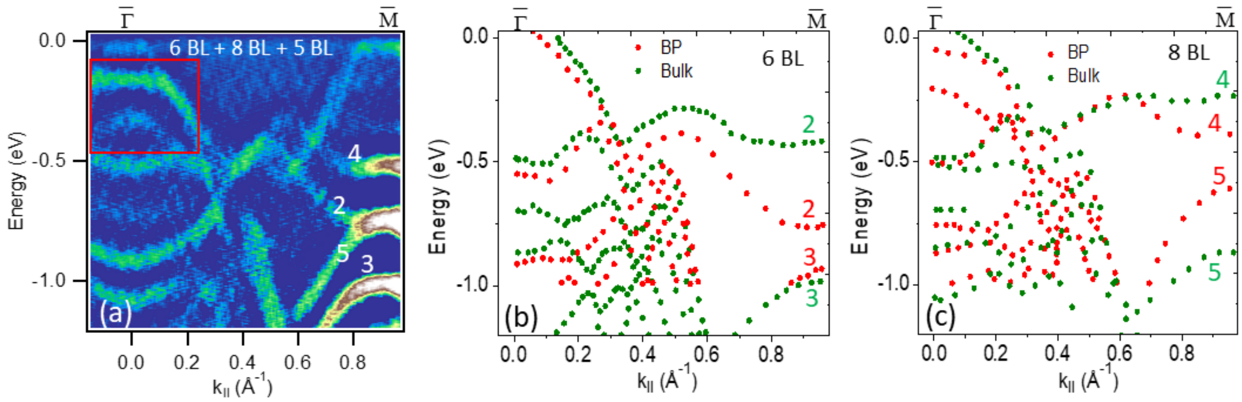


Figure S2. Comparison between experimental and theoretical dispersions along $\bar{\Gamma} - \bar{M}$ symmetry directions of Bi(110) SBZ accounting bulk-like A7 (Bulk) [8] and BP-like (BP) [24] Bi(110) films. (a) 2D derivative of band dispersions for 4 BL films. Theoretical dispersions for 6 BL (b) and 8 BL (c) Bi(110) films using bulk and BP-like structure. The states near the $\bar{M}$ point are marked by numbers, both in the experiment and calculations. Calculated states in red and green represent electronic states from BP and bulk-like structures, respectively. States within the red square in (a) can only be reproduced if 8 BL films have the BP structure.
